# Supplementary material for: The Muon Space GNSS-R Surface Soil Moisture Product
Source: arXiv:2412.00072 ancillary file (2024-11-26)
Supplement: Supplementary file 1 [file The_Muon_Space_GNSS_R_Surface_Soil_Moisture_Product_Supplemental.pdf]

# The Muon Space GNSS-R Surface Soil Moisture Product: Supplemental Materials

**Max Roberts[1,†*], Ian Colwell[1,†], Clara Chew[1,†], Dallas Masters[1], and Karl Nordstrom[1]**

[1]Muon Space, Science Team, 2250 Charleston Rd, Mountain View, CA 94043
[*]corresponding author: Max Roberts (max@muonspace.com)
[†]these authors contributed equally to this work

## Supplemental Comments/Figures

A water fraction study indicated that our initial selection of a MODIS-based mask was likely not the most representative option based on direct comparison to CYGNSS-derived reflectivity maps. Upon further inspection, it was apparent that the MODIS water mask is likely too coarse (250 m) to adequately mask out small open water bodies that GNSS-R observations sense. Figure 1 shows an illustration of the problem, where currently only observations with a water fraction > 0.01 are removed from the training dataset. As can be seen in Figure 1, there are clear rivers and small water bodies that are affecting the reflectivity observations that are not masked out using the current approach. Model testing with alternative, finer-resolution water masks is currently ongoing.

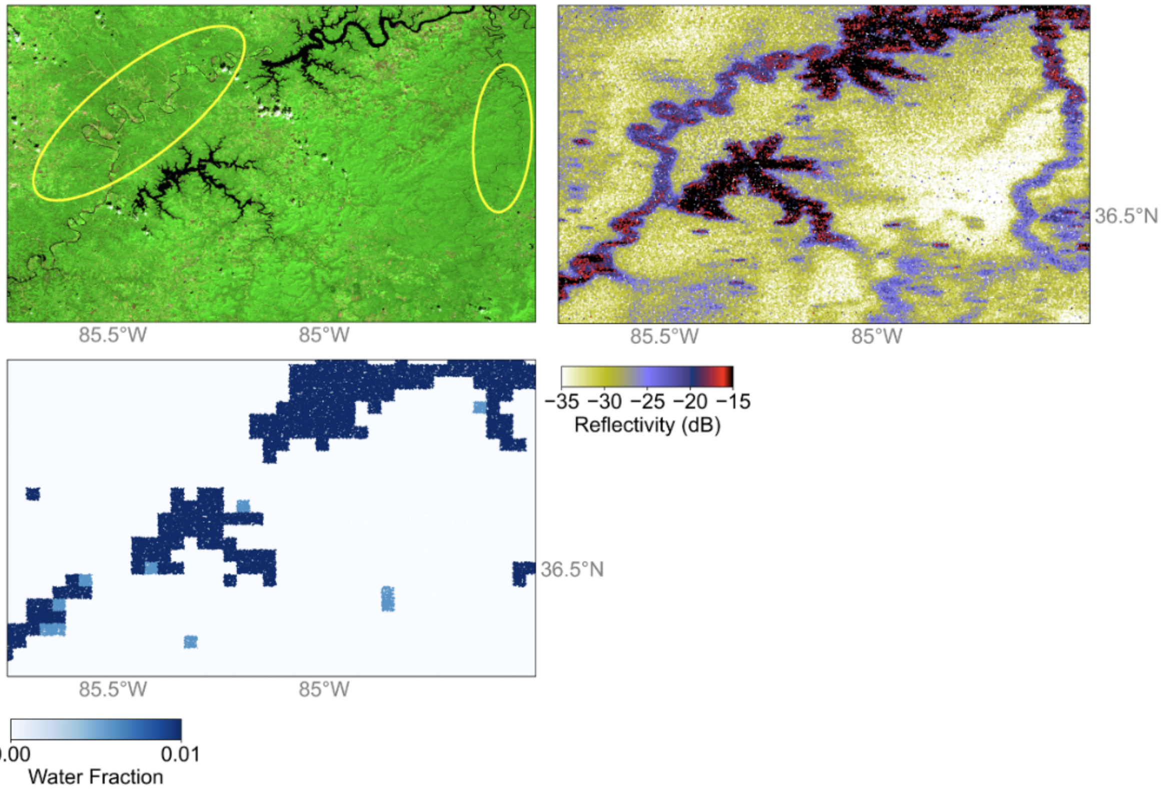


**Figure 1.** (top left) False color Sentinel-2 composite over a region in Tennessee. Yellow circles are rivers that strongly affect the reflected GNSS signal but are not included in the current water mask. (top right) Ungridded reflectivity observations for the same area. Note high reflectivity over the reservoirs and rivers shown in the Sentinel-2 image. (bottom left) Water fraction from MODIS, gridded to 3 km, which is used as the current water mask. The mask is too coarse to include the rivers that strongly affect the GNSS reflection.

A comparison of land cover based on a dominant type (single value, provided in SMAP ancillary), versus fractional representation of all types (17 element array) showed increase in model skill. This input was then used to derive an improved vegetation water content (VWC) value, which also showed additional improvement to model skill. Figure 2 shows the VWC maps before (top) and after (bottom) this update. Note that the smoother gradients and detailed structure visible in VWC are due to continuously varying fractional land cover type.

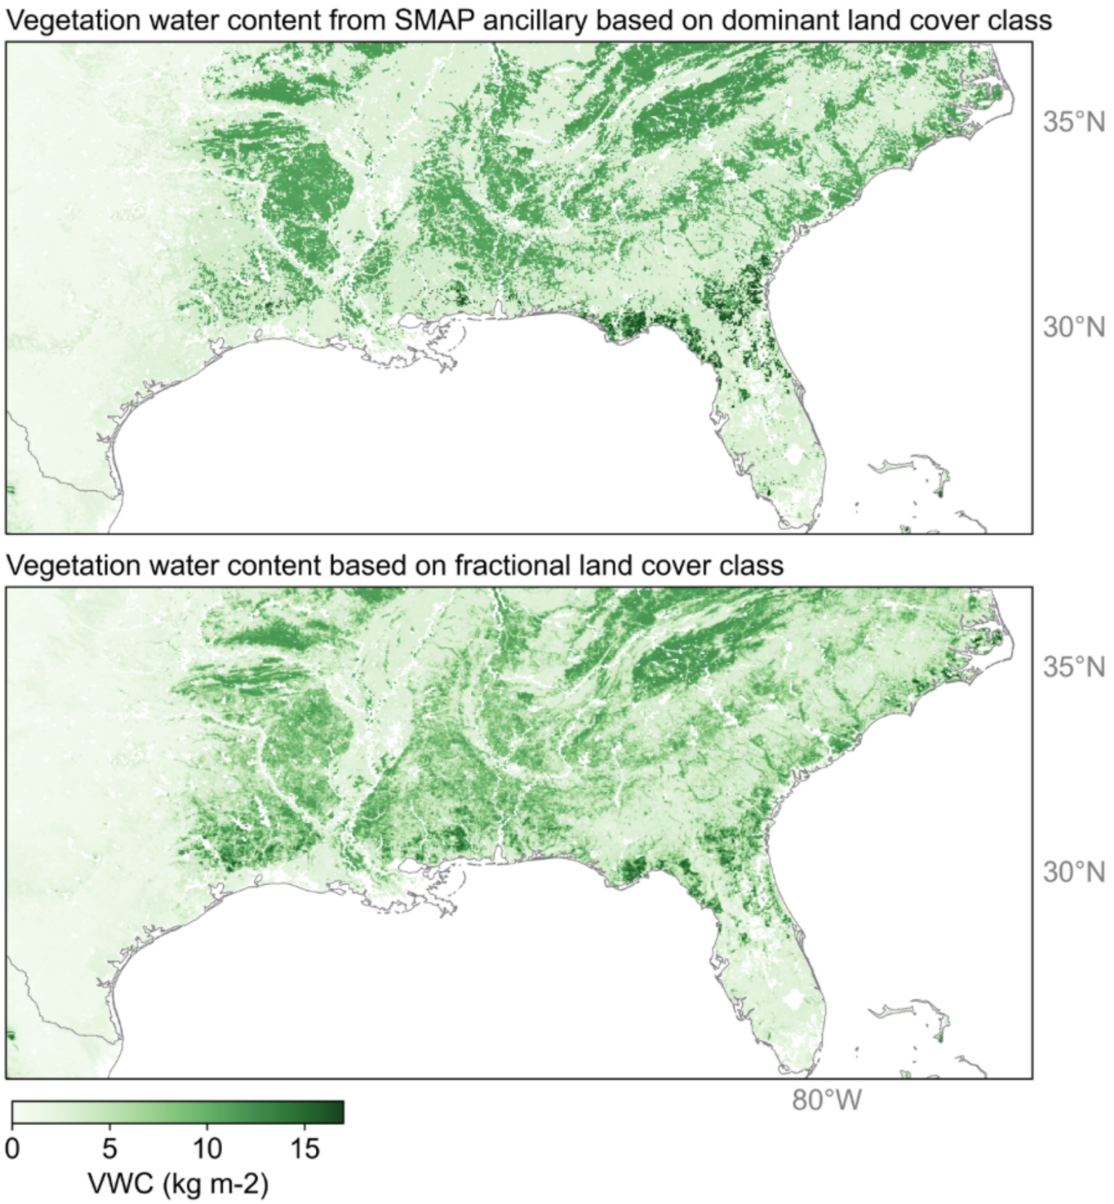


**Figure 2.** Vegetation water content derived using a climatology of NDVI and either the dominant IGBP land cover class in each 3 km grid cell (top) or using fractional IGBP land cover class (bottom).

| Filter | Description | Percent Samples removed |
|---|---|---|
| s_band_powered_up | CYGNSS flag | 0.70% |
| large_sc_attitude_err | CYGNSS flag | 0.10% |
| black_body_ddm | CYGNSS flag | 3.30% |
| ddmi_reconfigured | CYGNSS flag | 1.30% |
| spacewire_crc_invalid | CYGNSS flag | 0.00% |
| ddm_is_test_pattern | CYGNSS flag | 0.00% |
| large_step_lna_temp | CYGNSS flag | 0.00% |
| direct_signal_in_ddm | CYGNSS flag | 0.80% |
| low_confidence_gps_eirp_estimate | CYGNSS flag | 9.80% |
| brcs_ddm_sp_bin_delay_error | CYGNSS flag | 11.40% |
| brcs_ddm_sp_bin_dopp_error | CYGNSS flag | 3.70% |
| gps_pvt_sp3_error | CYGNSS flag | 0.00% |
| sp_non_existent_error | CYGNSS flag | 0.00% |
| brcs_lut_range_error | CYGNSS flag | 0.60% |
| ant_data_lut_range_error | CYGNSS flag | 7.30% |
| bb_framing_error | CYGNSS flag | 0.00% |
| fsw_comp_shift_error | CYGNSS flag | 0.00% |
| low_quality_gps_ant_knowledge | CYGNSS flag | 0.00% |
| sc_altitude_out_of_nominal_range | CYGNSS flag | 0.00% |
| incorrect_ddmi_antenna_selection | CYGNSS flag | 7.00% |
| sp_in_sidelobe | CYGNSS flag | 8.50% |
| fatal_nst_outage | CYGNSS flag | 2.00% |
| low_zenith_ant_gain | CYGNSS flag | 7.70% |
| poor_bb_quality | CYGNSS flag | 4.40% |
| poor_quality_bin_ratio | CYGNSS flag | 6.50% |
| low_coherency_ratio | CYGNSS flag | 9.60% |
| ddm_snr_lim | DDM SNR threshold (> 1) | 32.00% |
| elevation_lim | Surface elevation threshold (>3000 m) | 6.00% |
| gain_lim | Receiver gain threshold (> 1) | 17.00% |
| incidence_lim | Specular point incidence angle threshold (> 65°) | 6.00% |
| water_frac_lim | Surface water fraction at specular point (< 1% of 3 km) | 5.00% |
| target_quality_flags | SMAP quality flags (must be at least “successful”) | 64.00% |
| target_surface_flags | SMAP surface flags (removes target data with rain/snow) | 1.20% |

**Table 1.** Flag filtering statistics computed for CYG03 for all of 2021. Note that the numbers here are not mutually exclusive and should not be tallied.

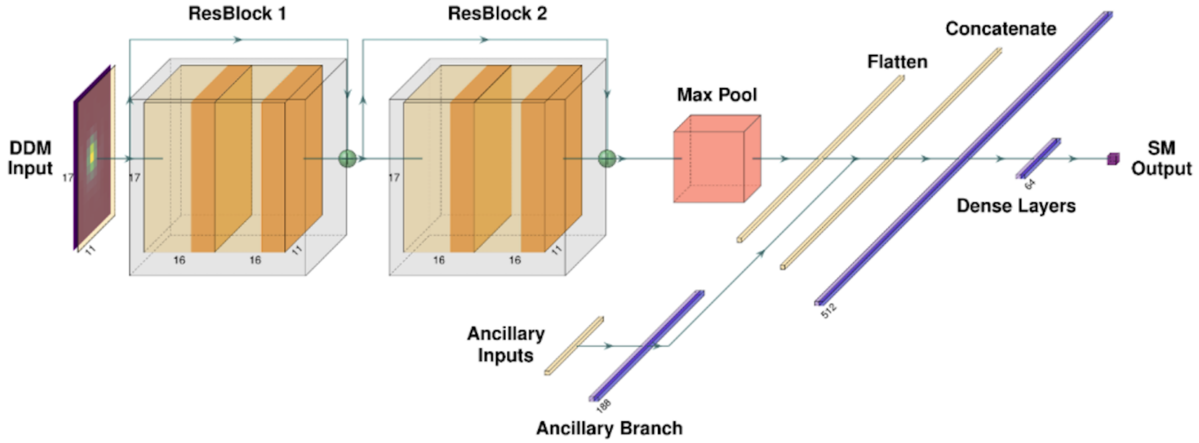


**Figure 3.** High-level diagram of the CNN-based architectures developed for generalized GNSS-R retrievals, and applied to SM. Convolutional layers perform learned feature extraction from input data, those learned features are flattened and passed to dense layers. The convolutional layers wrapped in Residual Blocks which include skip connections. A separate dense layer handles ancillary inputs prior to concatenating with the ResBlock outputs and being passed to the dense layers.

| Variable | Description | Units |
|---|---|---|
| time | Seconds since midnight UTC on the start of the day of collection | s |
| lat | Latitude of the specular reflection point | degree north |
| lon | Longitude of the specular reflection point | degree east |
| soil_moisture_level2 | Soil moisture retrieval | m3 m-3 |
| elevation | Average surface elevation of the 3-km EASE grid cell containing the specular reflection point. | m |
| elevation_std | Standard deviation of elevation of the 3-km EASE grid cell containing the specular reflection point. | m |
| slope | Average slope of the 3-km EASE grid cell containing the specular reflection point. | degree |
| slope_std | Standard deviation of slope of the 3-km EASE grid cell containing the specular reflection point. | degree |
| normalized_vegetation_ difference_index | The ratio of red and near infrared bands in optical remote sensing data, used to indicate vegetation greenness. | unitless |
| fractional_vegetation_water _content_ndvi | Vegetation water content within the 3-km grid cell containing the specular reflection point based on the normalized difference vegetation index. | kg m-2 |
| fractional_land_cover_class | Fraction of each 3-km grid cell containing the specular reflection point that is a particular IGBP land cover class. | unitless |
| surface_roughness | RMS of small-scale surface height deviations, parameterized from land cover class. | m |
| bulk_density | Weight of dry soil relative to its volume | kg m-3 |
| clay_fraction | Fraction of surface soil layer that is composed of clay. | unitless |
| sand_fraction | Fraction of surface soil layer that is composed of sand. | unitless |
| water_fraction | Fraction of 3-km EASE grid cell that contains open water. | unitless |
| channel | Channel that recorded the GNSS reflection. | unitless |
| sc_pos_x | The X component of the spacecraft WGS84 reference frame ECEF position. | m |
| sc_pos_y | The Y component of the spacecraft WGS84 reference frame ECEF position. | m |
| sc_pos_z | The Z component of the spacecraft WGS84 reference frame ECEF position. | m |
| sc_vel_x | The X component of the spacecraft WGS84 reference frame ECEF velocity. | m/s |
| sc_vel_y | The Y component of the spacecraft WGS84 reference frame ECEF velocity. | m/s |
| sc_vel_z | The Z component of the spacecraft WGS84 reference frame ECEF velocity. | m/s |
| sc_roll | Spacecraft roll angle relative to the orbit frame. | radians |
| sc_pitch | Spacecraft pitch angle relative to the orbit frame. | radians |
| sc_yaw | Spacecraft yaw angle relative to the orbit frame. | radians |
| sc_lat | Subsatellite point latitude | degree north |
| sc_lon | Subsatellite point longitude | degree east |
| sc_alt | Spacecraft altitude above the WGS84 ellipsoid | m |
| prn_code | The PRN code of the GNSS signal associated with the DDM. | unitless |
| sv_num | The GPS unique space vehicle number that transmitted the PRN code. | unitless |
| tx_pos_x | The X component of the GPS spacecraft WGS84 reference frame ECEF position. | m |
| tx_pos_y | The Y component of the GPS spacecraft WGS84 reference frame ECEF position. | m |
| tx_pos_z | The Z component of the GPS spacecraft WGS84 reference frame ECEF position. | m |
| gps_eirp | The effective isotropic radiated power of the GNSS space vehicle in the direction of the spacecraft. | unitless |
| sp_rx_gain | The receive antenna gains in the direction of the specular point. | dB |
| sp_rx_range | The distance between the spacecraft and the specular point. | m |
| tx_sp_range | The distance between the GNSS spacecraft and the specular point. | m |
| ddm_ant | The antenna that received the reflected GNSS signal associated with the DDM. | unitless |
| sp_inc_angle | The specular point incidence angle. | degrees |
| theta | Theta angle to the specular point. | degrees |
| azimuth | Azimuth angle to the specular point. | degrees |
| ddm_snr | 10log(Smaxr/Navg), where Smaxr is the maximum value (in counts) in a single DDM bin, and Navg is the average per-bin raw noise counts. | dB |
| reflectivity | Smax corrected for antenna gain, transmit power, and range, assuming coherent reflections, where Smax is the maximum value in a single DDM bin. | unitless |
| ddm_noise_floor | Equal to the average bin raw counts in the first 45 delay rows of the uncompressed DDM, in counts. | unitless |
| ddm_qual_flag_lhcp | Per-DDM quality flags. 1 indicates the presence of the condition. | unitless |
| soil_moisture_level2_error | Soil moisture retrieval uncertainty. | m3 m-3 |
| retrieval_qual_flag | Bit flags that record the conditions and the quality of the soil moisture retrieval per observation. | unitless |
| surface_flag | Bit flag that records ambient surface conditions for the observation. | unitless |
| SPL3SMP_E | SMAP Enhanced L3 Radiometer-based soil moisture retrieval, version 5. | m3 m-3 |

**Table 2.** Contents of L2 product files.

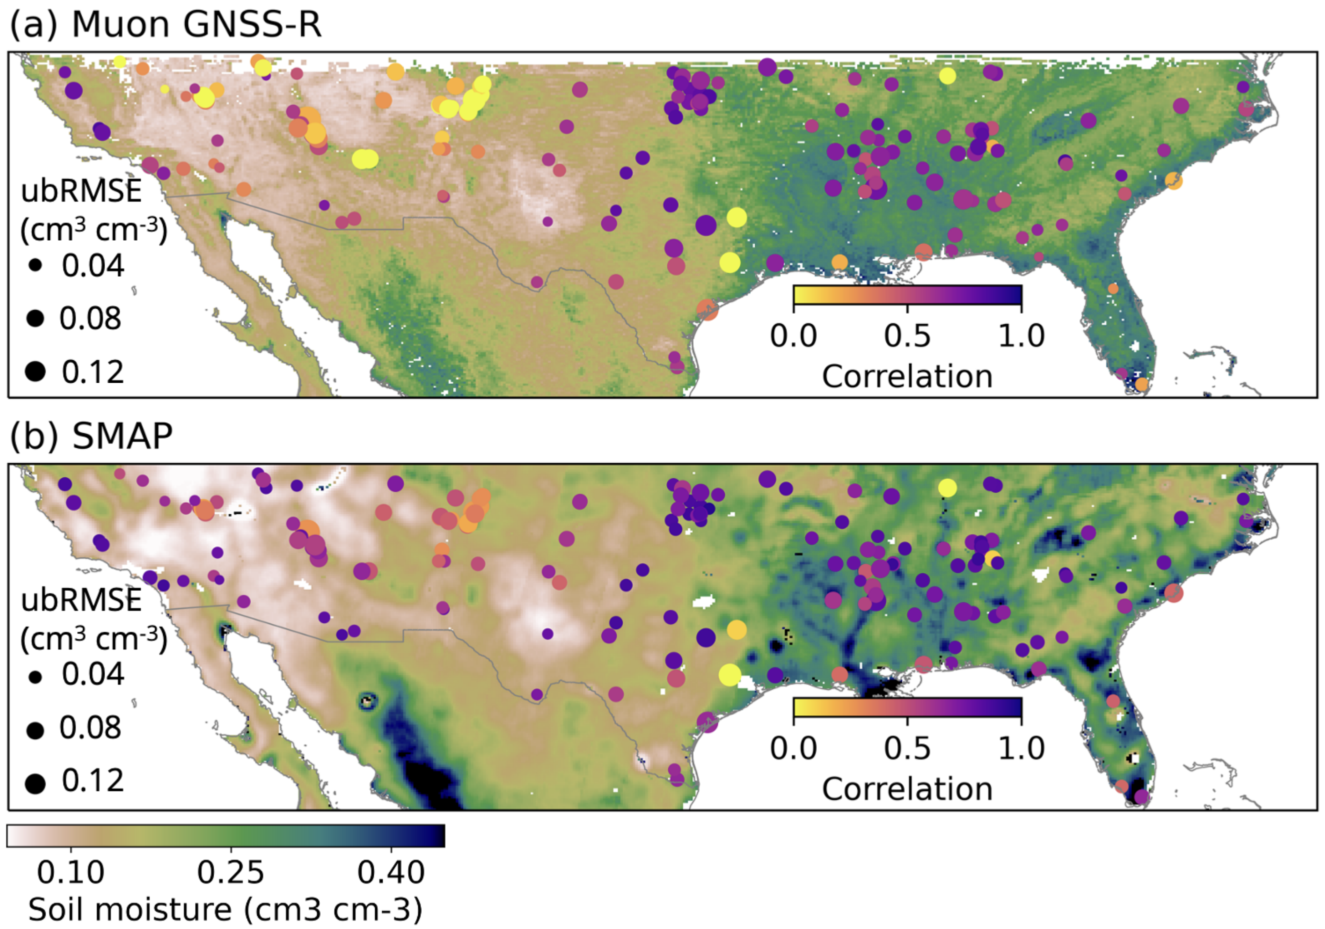


**Figure 4.** Same as manuscript Figure 8, except showing the validation statistics for the Level 3 Muon GNSS-R product and the SMAP Enhanced Product, gridded to 9 km.

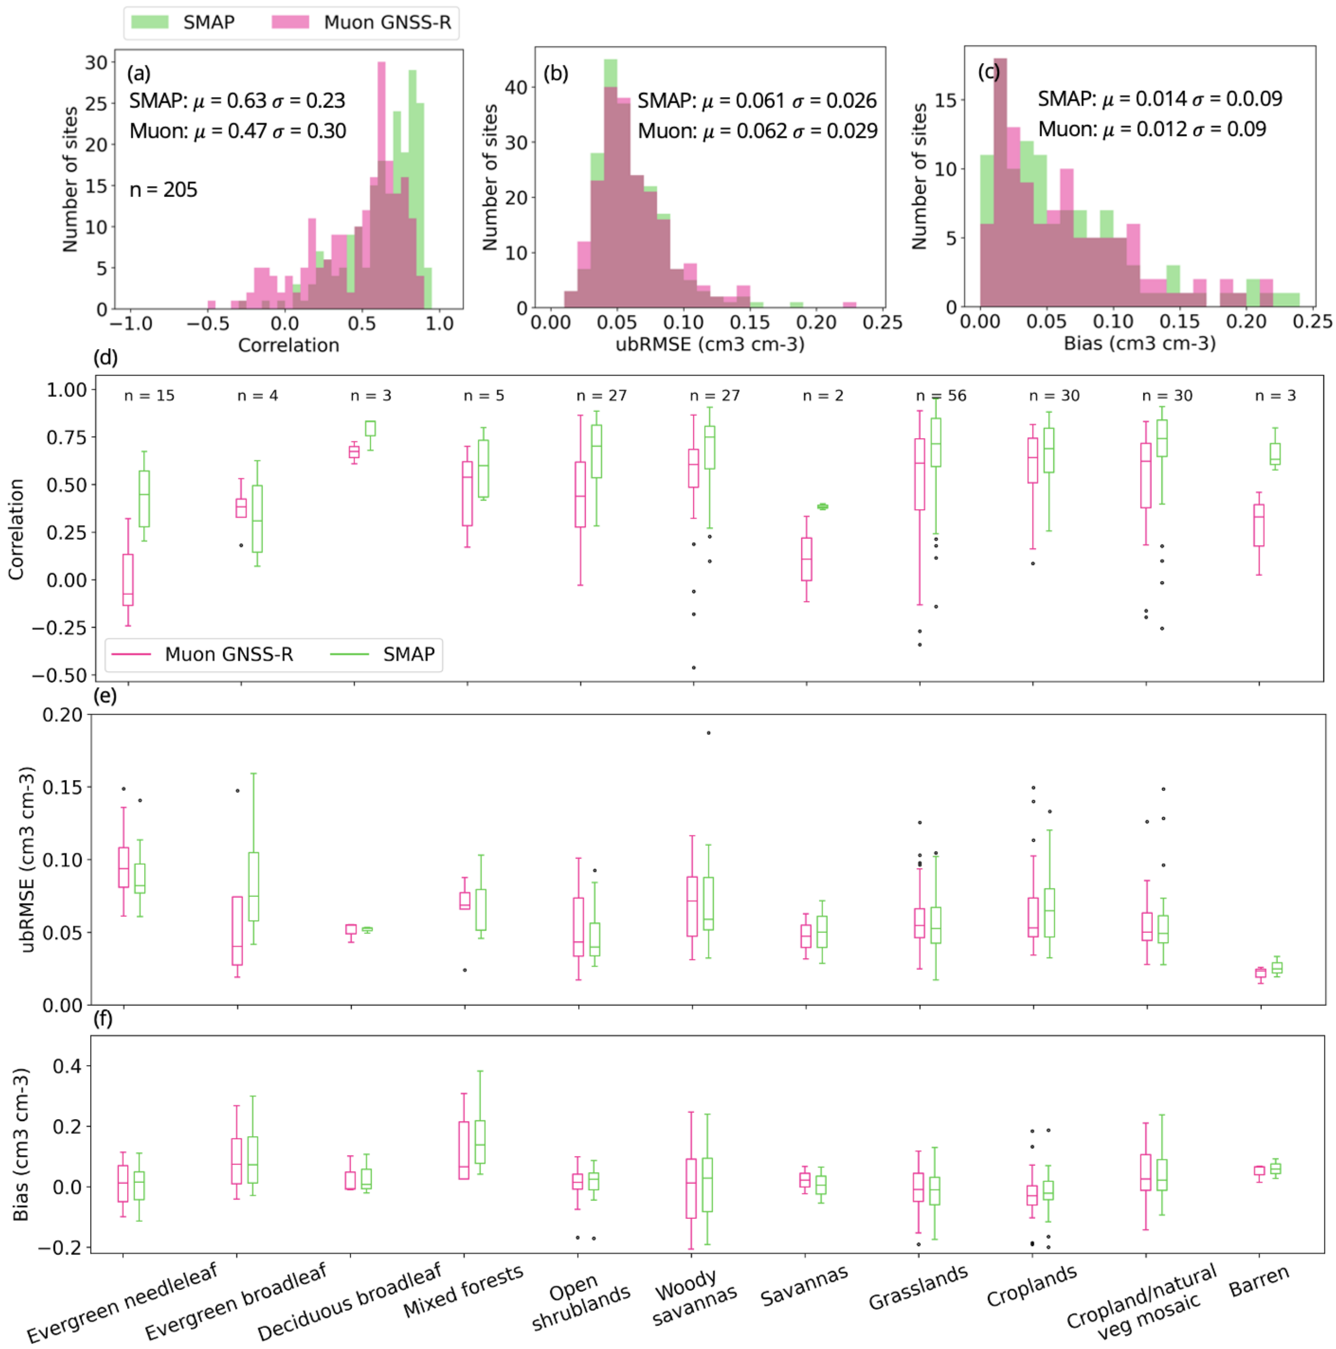


**Figure 5.** Same as manuscript Figure 9, except showing statistics for the Level 3 Muon GNSS-R retrievals and the SMAP Enhanced Product, gridded to 9 km.

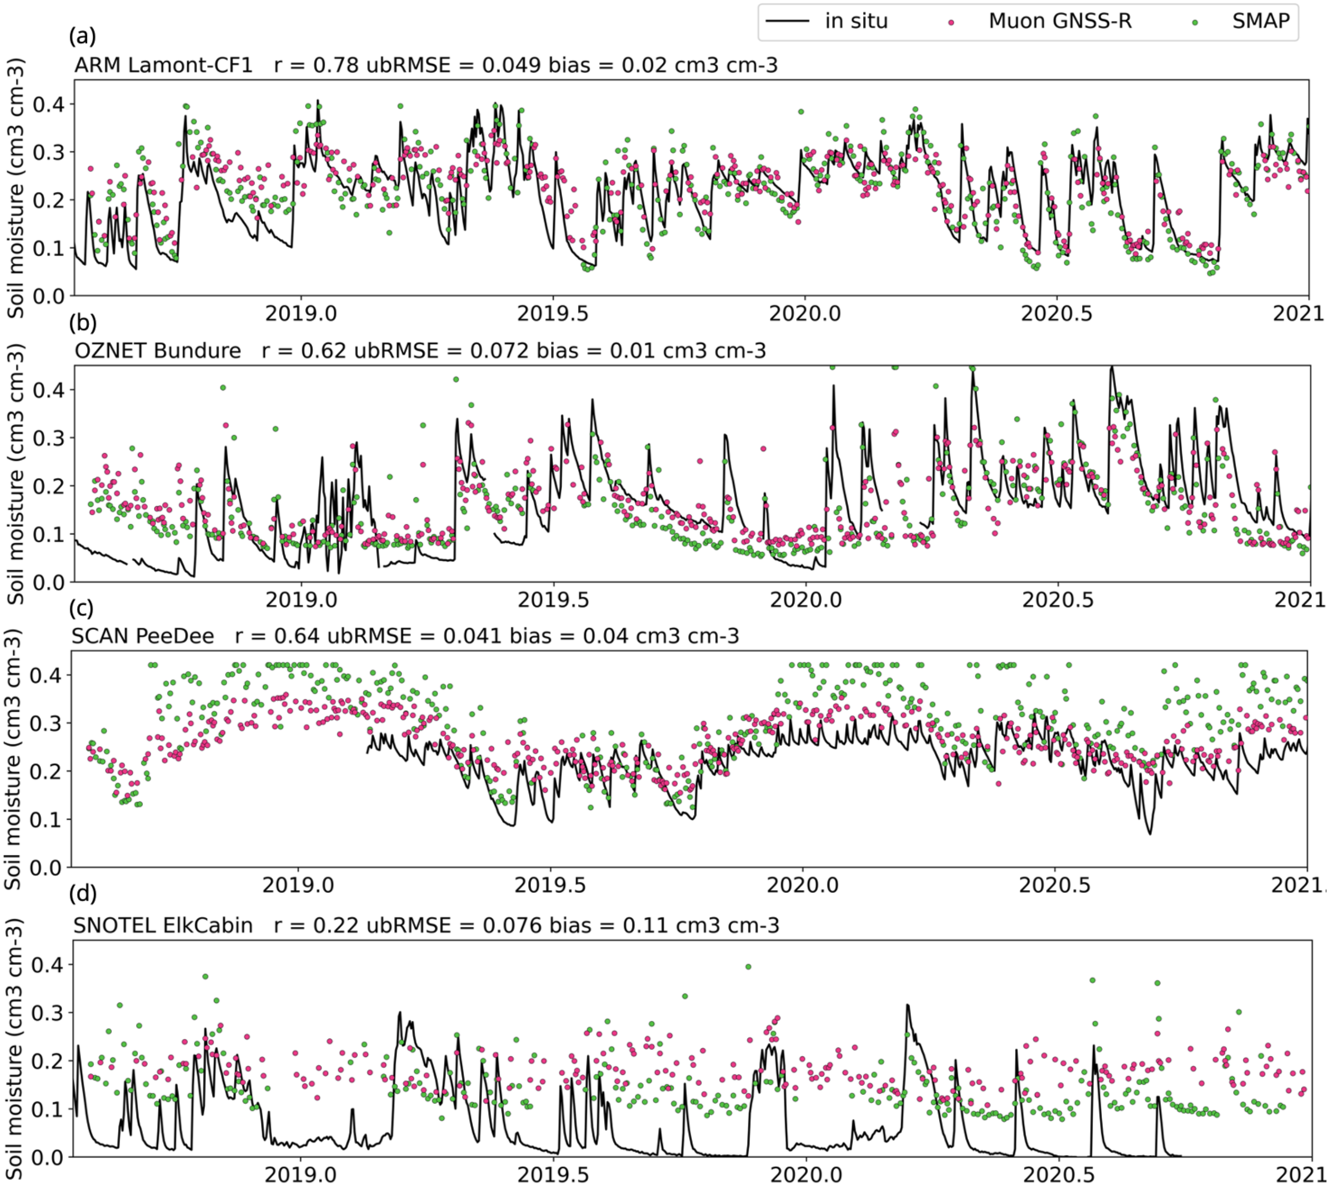


**Figure 6.** The same time series as shown in manuscript Figure 10, except showing the Level 3 Muon GNSS-R retrievals and the SMAP Enhanced Product at 9 km.

| | **Correlation** | | **ubRMSE (cm3 cm-3)** | | **Bias (cm3 cm-3)** | |
|---|---|---|---|---|---|---|
| **Site Name** | Muon GNSS-R | SMAP | Muon GNSS-R | SMAP | Muon GNSS-R | SMAP |
| 0701 Yanco | 0.74 | 0.79 | 0.044 | 0.045 | 0.05 | 0.03 |
| 1601 Walnut Gulch | 0.3 | 0.7 | 0.036 | 0.033 | 0.02 | 0.02 |
| 1602 Little Washita | 0.81 | 0.95 | 0.026 | 0.02 | 0.01 | 0.01 |
| 1603 Fort Cobb | 0.78 | 0.9 | 0.036 | 0.03 | -0.02 | -0.02 |
| 1604 Little River | 0.61 | 0.77 | 0.036 | 0.047 | 0.1 | 0.1 |
| 1902 MonteBuey | 0.72 | 0.83 | 0.036 | 0.033 | -0.01 | -0.02 |
| 4801 TxSON | 0.75 | 0.93 | 0.036 | 0.026 | 0 | 0 |
| Mean of all | 0.67 | 0.84 | 0.036 | 0.033 | 0.02 | 0.02 |

**Table 3.** Validation statistics for the L3 Muon GNSS-R retrievals and the SMAP Enhanced Product, gridded to 9 km, at the SMAP Core Validation sites within the latitudinal band of CYGNSS.

## Supplemental Material on Gridding

The equal weighting approach is a simple average of all retrievals for which the specular reflection point falls within a grid cell. Nearest neighbor only considers the retrieval closest to the grid cell center, and all other retrievals are thrown out. Inverse distance weighting is a compromise between equal weighting and nearest neighbor: although all retrievals are considered, retrievals closer to the grid cell center are weighted more heavily than those closer to the grid cell edges. In order to test this approach, we used the same weighting criteria as SMAP where the weights are inversely proportional to the square of the great circle distance from the grid cell center. More details can be found here:

https://nsidc.org/sites/nsidc.org/files/files/279_L1C_TB_ATBD_RevA_web.pdf

Very little appreciable differences were noted between the resulting gridded retrievals using any one of the three approaches, though the equal weighting/drop-in-bucket method overall outperformed nearest neighbor and inverse distance weighting, with nearest neighbor performing the worst of the three methods. Figure 4 shows differences in validation statistics for products generated using the three different gridding methods for sparse network sites in CONUS.

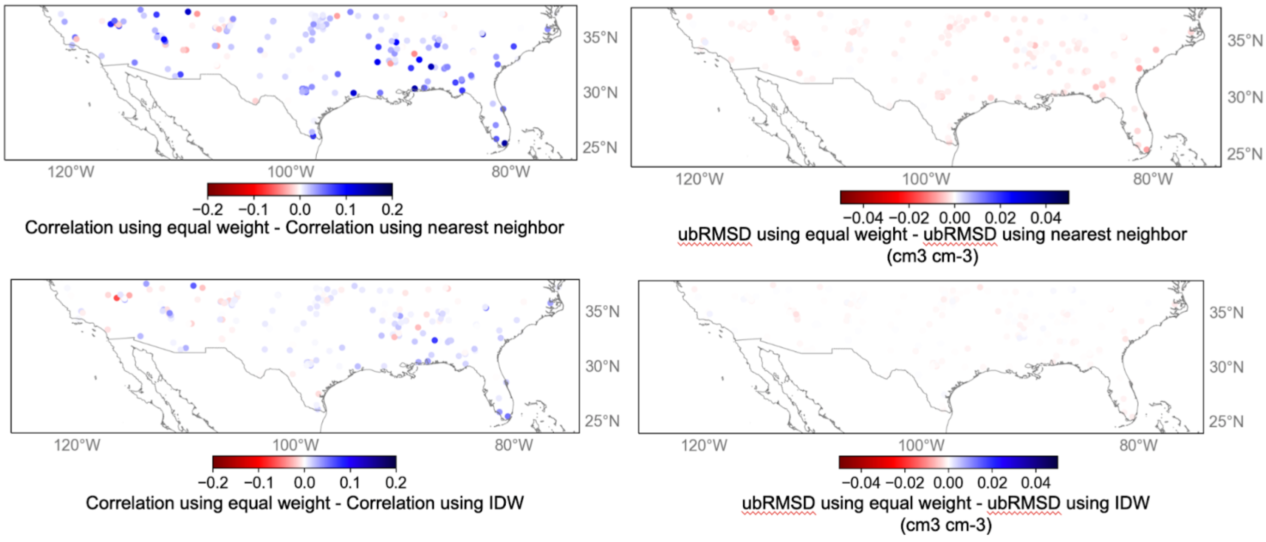


**Figure 7.** (top left) Difference in correlation at sparse network sites for gridded retrievals using the equal weighting method versus nearest neighbor. (top right) Same as top left, but showing unbiased root mean square differences (ubRMSD). (bottom left) Same as top left, but showing the correlation difference between equal weighting and IDW. (bottom right) Same as bottom left but showing ubRMSD.

The SM time series themselves generated using the three gridding methods often did not visually look appreciably different (e.g., Figure 5). This makes sense, given how few retrievals are generally averaged within each grid cell, usually between 0-5 observations, but most often 2-3. We hypothesize that equal weighting performed the best given the relative uncertainty between individual reflectivity observations that drive the retrieval model: averaging multiple uncertain values will decrease the amount of noise present relative to using only one value. As equal weighting slightly outperformed the other two gridding methods, our hourly retrievals use this type of gridding method to derive grid cell averages.

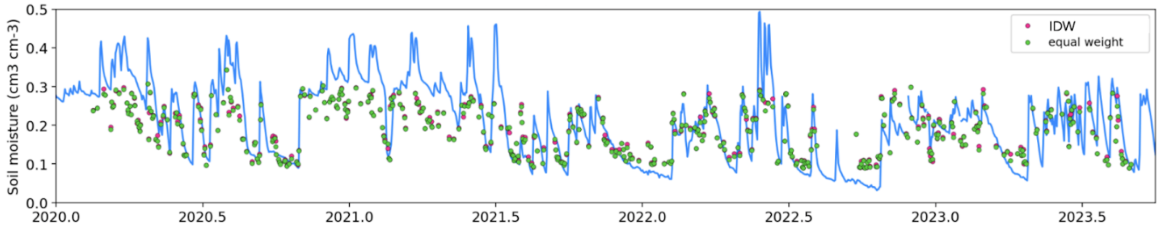


**Figure 8.** SM time series at one sparse network site illustrating the typical small differences in retrievals regardless of gridding method.
